# Supplementary material for: Bridging Swift Error Handling Model to C++
Source: arXiv:2301.10353 source file (2023-01-24)
Supplement: Supplementary file 1 [file appendice.tex]

We have known some people that have worn the ring in the past. They are described in Table \ref{tab:ring_and_age}

\begin{table}[hb]
\centering
\begin{tabular}{cc}
\hline
Name    & Age       \\ \hline
Frodo   & 51        \\
Boromir & 41        \\
Smeagol & $\sim$600 \\ \hline
\end{tabular}
\caption{The age (in years) of people that have worn the ring}
\label{tab:ring_and_age}
\end{table}
